# Supplementary material for: High contrast dual-mode optical and 13C magnetic resonance imaging in diamond particles
Source: arXiv:1909.08064 source file (2021-04-04)

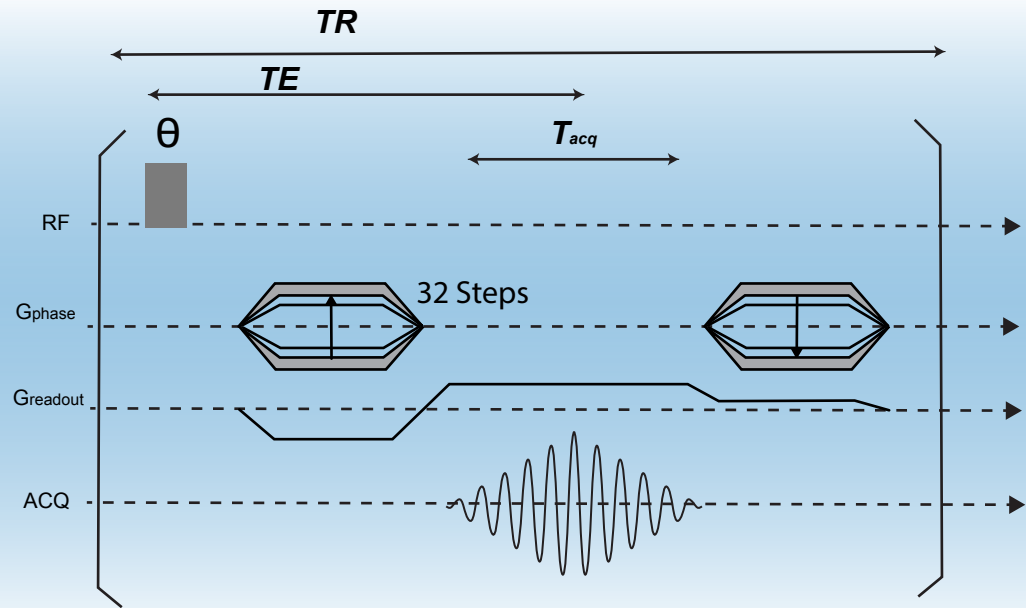

Supplement: Supplementary file 2 [file imaging_sequence-2.pdf]
