# Supplementary material for: High contrast dual-mode optical and 13C magnetic resonance imaging in diamond particles
Source: arXiv:1909.08064 source file (2021-04-04)
Supplement: Supplementary file 3 [file Commands3.tex]

\newcommand{\inset}{\hspace{10pt}}
\newcommand{\vs}{\vspace{10pt}}
% Math symbols
\newcommand{\itwo}{{\frac1{2}}}
\newcommand{\ist}{{\frac1{\sqrt{2}}}}
\newcommand{\id}{\mathds{1}}
\newcommand{\half}{\frac{1}{2}}
% Greek small
\newcommand{\xa}{\alpha}
\newcommand{\cc}{{\cal C}}
\newcommand{\hb}{\hbar}
\newcommand{\xb}{\beta}
\newcommand{\xc}{\chi}
\newcommand{\xd}{\delta}
\newcommand{\xe}{\epsilon}
\newcommand{\angstrom}{\mbox{\normalfont\AA}}

%\newcommand{\xe}{\upvarepsilon}
\newcommand{\xg}{\gamma}
\newcommand{\xt}{\theta}
\newcommand{\ot}{\otimes}
\newcommand{\xn}{\eta}
\newcommand{\xk}{\kappa}
\newcommand{\xl}{\lambda}
\newcommand{\xr}{\rho}
\newcommand{\xo}{\omega}
\newcommand{\xph}{\phi}
\newcommand{\xps}{\psi}
\newcommand{\nb}{\nabla}
\newcommand{\xvph}{\varphi}
\newcommand{\xs}{\sigma}
\newcommand{\xz}{\zeta}
\newcommand{\pp}{\perp}
\newcommand{\app}{\approx}
\newcommand{\dw}{\downarrow}
\newcommand{\up}{\uparrow}
\newcommand{\Cs}{{}^{13}\R{C}}
\newcommand{\Ns}{{}^{14}\R{N}}
\newcommand{\Hs}{{}^{1}\R{H}}

\newcommand{\mG}[0]{\mathcal{G}}
\newcommand{\mR}[0]{\mathcal{R}}
\newcommand{\bB}[0]{\mathbf B}
\newcommand{\bs}[0]{\mathbf \sigma}
\newcommand{\bH}[0]{\mathbf H}
\newcommand{\bn}[0]{\hat{\mathbf n}}

\newcommand{\ltrt}{\leftrightarrow}
\newcommand{\iso}[1]{{}^{#1}}
\newcommand{\V}[1]{\vec{#1}}
%\newcommand{\mc}[1]{\mathcal{#1}}

\newcommand{\sinc}{\R{sinc}}
\newcommand{\rect}{\R{rect}}

\newcommand{\spl}[1]{\begin{align}\begin{split} #1 \end{split} \end{align}}

% Greek large
\newcommand{\xA}{\Alpha}
\newcommand{\xB}{\Beta}
\newcommand{\xD}{\Delta}
\newcommand{\xE}{\Epsilon}
\newcommand{\xG}{\Gamma}
\newcommand{\xT}{\Theta}
\newcommand{\xN}{\Eta}
\newcommand{\xK}{\Kappa}
\newcommand{\xL}{\Lambda}
\newcommand{\xO}{\Omega}
\newcommand{\xPh}{\Phi}
\newcommand{\xPs}{\Psi}
\newcommand{\xS}{\Sigma}
\newcommand{\Spl}[1]{\begin{align*}\begin{split} #1 \end{split} \end{align*}}


\newcommand{\mP}[0]{\mathcal{P}}
\newcommand{\mU}[0]{\mathcal{U}}
\newcommand{\bp}[0]{\mathbf p}
\newcommand{\bq}[0]{\mathbf q}
\newcommand{\bP}[0]{\mathbf P}
\newcommand{\bb}[0]{\mathbf b}

\newcommand{\bA}[0]{\mathbf A}
\newcommand{\bS}[0]{\mathbf S}
\newcommand{\bI}[0]{\mathbf I}
%\newcommand{\bB}[0]{\mathbf B}
\newcommand{\bxO}[0]{\mathbf \Omega}
\newcommand{\bM}[0]{\mathbf M}
\newcommand{\be}[0]{\mathbf e}
\newcommand{\bu}[0]{\mathbf u}
\newcommand{\bv}[0]{\mathbf v}
\newcommand{\bR}[0]{\mathbf R}
\newcommand{\bx}[0]{\hat{\mathbf x}}
\newcommand{\by}[0]{\hat{\mathbf y}}
\newcommand{\bz}[0]{\hat{\mathbf z}}
\newcommand{\br}[0]{\hat{\mathbf r}}
\newcommand{\balpha}[0]{\boldsymbol \alpha}
\newcommand{\bdelta}[0]{\boldsymbol \delta}
\newcommand{\al}[1]{\begin{align} #1 \end{align}}

% other useful commands
\newcommand{\fr}[2]{\frac{#1}{#2}}
\newcommand{\ov}[1]{\overline{#1}}
\newcommand{\wt}[1]{\widetilde{#1}}
\newcommand{\dwt}[1]{\widetilde{\widetilde{#1}}}
\newcommand{\h}[1]{\hat{#1}}
\newcommand{\s}[2]{\sum_{#1}^{#2}}
\newcommand{\zi}[2]{\int_{#1}^{#2}}
\newcommand{\sq}[1]{\sqrt{#1}}
\newcommand{\zd}{\cdot}

\newcommand{\mH}[0]{\mathcal{H}}
\newcommand{\mF}[0]{\mathcal{F}}
\newcommand{\mT}[0]{\mathcal{T}}
\newcommand{\mB}[0]{\mathcal{B}}

\newcommand{\rt}{\rightarrow}
\newcommand{\lt}{\leftarrow}
\newcommand{\xrt}[1]{\xrightarrow{#1}}
\newcommand{\Rt}{\Rightarrow}
\newcommand{\xinf}{\infty}
\newcommand{\op}{\oplus}
\newcommand{\oti}{\otimes}
\newcommand{\e}{\exp}
\newcommand{\dg}{\dagger}

\newcommand{\beq}{\begin{equation}}
\newcommand{\eeq}{\end{equation}}
                  
\newcommand{\benum}{\begin{enumerate}}
\newcommand{\eenum}{\end{enumerate}}
                    
\newcommand{\bit}{\begin{itemize}}
\newcommand{\eit}{\end{itemize}}


\newcommand{\bea}{\begin{eqnarray}}
\newcommand{\eea}{\end{eqnarray}}

\newcommand{\bev}{\begin{verbatim}}
\newcommand{\eev}{\end{verbatim}}

\newcommand{\code}[1]{\texttt{#1}}

\newcommand{\non}{\nonumber}
\newcommand{\noi}{\noindent}
\newcommand{\cd}{\cdots}
\newcommand{\zt}{\times}

\newcommand{\qt}{\tau}

% brackets
\newcommand{\lb}{\left(}
\newcommand{\rb}{\right)}
\newcommand{\lsb}{\left[}
\newcommand{\rsb}{\right]}
\newcommand{\lcb}{\left\{}
\newcommand{\rcb}{\right\}}
\newcommand{\labs}{\left|}
\newcommand{\rabs}{\right|}
\newcommand{\lan}{\langle}
\newcommand{\ran}{\rangle}
\newcommand{\pll}{\parallel}
\newcommand{\ppp}{\perp}
\newcommand{\Rb}{${}^{87}$Rb\ }

%bold
\newcommand{\B}[1]{\mathbf{#1}}
\newcommand{\T}[1]{\textbf{#1}}
\newcommand{\I}[1]{\textit{#1}}
\newcommand{\R}[1]{\textrm{#1}}
%\newcommand{\Ir}[1]{\textit{\Rd{#1}}}
\newcommand{\IIr}[1]{\textit{\Rd{#1}}}

%\newcommand{\C}{\cdot}
\newcommand{\vv}{\vec}
\newcommand{\dov}[1]{\overline{\overline{#1}}}

%label and ref
\newcommand{\zl}[1]{\label{eqn:#1}}
\newcommand{\zr}[1]{Eq. (\ref{eqn:#1})}
\newcommand{\zfl}[1]{\protect\label{fig:#1}}
\newcommand{\zfr}[1]{Fig. \ref{fig:#1}}
\newcommand{\ztl}[1]{\label{table:#1}}
\newcommand{\ztr}[1]{Table \ref{table:#1}}
\newcommand{\zsl}[1]{\label{sec:#1}}
\newcommand{\zsr}[1]{Sec. \ref{sec:#1}}
\newcommand{\zal}[1]{\label{app:#1}}
\newcommand{\zar}[1]{Appendix \ref{app:#1}}




% For NV
\newcommand{\carb}{$^{13}$C }
% Quantum Kets
\newcommand{\ket}[1]{\left\vert{#1}\right\rangle}
\newcommand{\bra}[1]{\left\langle{#1}\right\vert}
\newcommand{\braket}[2]{\langle{#1}\vert{#2}\rangle}
\newcommand{\ketbra}[2]{\ket{#1}\bra{#2}}
\newcommand{\sand}[3]{\langle{#1}\vert#2\vert{#3}\rangle}
\newcommand{\expec}[1]{\left\langle #1\right\rangle}
\newcommand{\kpsi}{\vert{\psi}\rangle}
\newcommand{\kphi}{\vert{\phi}\rangle}
\newcommand{\kphit}{\vert{\phit}\rangle}
\newcommand{\bpsi}{\langle{\psi}\vert}
\newcommand{\bphi}{\langle{\phi}\vert}
\newcommand{\bphit}{\langle{\phit}\vert}
\newcommand{\ku}{\vert{0}\rangle}
\newcommand{\kd}{\vert{1}\rangle}
\newcommand{\kup}{\vert{\uparrow}\rangle}
\newcommand{\kdw}{\vert{\downarrow}\rangle}
%\newcommand{\bu}{\langle{0}\vert}
%\newcommand{\bd}{\langle{1}\vert}
\newcommand{\kk}{\vert{k}\rangle}
\newcommand{\bk}{\langle{k}\vert}
\newcommand{\ci}{\circ}
% Quantum Ops
\newcommand{\ave}[1]{\left\langle #1\right\rangle}
\newcommand{\vop}[1]{\hat{\vec{#1}}}
\newcommand{\comm}[2]{\left[{#1},{#2}\right]}
\newcommand{\ham}{{\mathcal{H}}}
%Pauli
\newcommand{\sone}{\mathds{1}}
\newcommand{\sx}{\sigma_x}
\newcommand{\sy}{\sigma_y}
\newcommand{\sz}{\sigma_z}
%\newcommand{\spl}{\sigma_+}
\newcommand{\sm}{\sigma_-}
% 2x2 Matrix
\newcommand{\mat}[4]{\left(\begin{array}{cc}{#1}&{#2}\\
{#3}&{#4}\end{array}\right)}
\newcommand{\matnob}[4]{\begin{array}{cc}{#1}&{#2}\\
{#3}&{#4}\end{array}}

\newcommand{\matthree}[9]{\left(\begin{array}{ccc}{#1}&{#2}&{#3}\\
{#4}&{#5}&{#6}\\
{#7}&{#8}&{#9}\end{array}\right)}

\newcommand{\ba}{\left\{ \begin{array}{lr}}
\newcommand{\ea}{\end{array}\right.}    

\newcommand{\coltwo}[2]{\left[\begin{array}{c}{#1}\\{#2}\end{array}\right]}


\newcommand{\diagfour}[4]{\left[\begin{array}{cccc}{#1}&{}&{}&{}\\
{}&{#2}&{}&{}\\
{}&{}&{#3}&{}\\
{}&{}&{}&{#4}
\end{array}\right]}

\newcommand{\diagthree}[3]{\left[\begin{array}{ccc}{#1}&{}&{}\\
{}&{#2}&{}\\
{}&{}&{#3}
\end{array}\right]}

\newcommand{\sect}[1]{\vspace{0.2in}
\noi\textbf{#1:\\}}             
 
%\newcommand{\bookjun}[1]{\href[page=#1]{../../notes/research/book-jun-2015.pdf}{Jun, page #1}}.
%\newcommand{\bookmay}[1]{\href[page={#1}]{../../notes/research/book-may-2015.pdf}{May, page {#1}}}.

\newcommand{\Bl}[1]{\textcolor{RoyalBlue}{#1}} %RoyalBlue MidnightBlue
\newcommand{\Rd}[1]{\textcolor{BrickRed}{#1}} %RoyalBlue MidnightBlue
%\newcommand{\Rd}[1]{\textcolor{Red}{#1}} %RoyalBlue MidnightBlue

% Trace
\newcommand{\Tr}[1]{\textrm{Tr}\left\{{#1}\right\}}
\newcommand{\tr}[1]{\textrm{Tr}\left\{{#1}\right\}}
\newcommand{\ptr}[2]{\textrm{Tr}_{#1}\left\{{#2}\right\}}
\newcommand{\pTr}[2]{\textrm{Tr}_{#1}\left\{{#2}\right\}}
\newcommand{\im}[1]{\textrm{Im}\left[{#1}\right]}
\newcommand{\re}[1]{\textrm{Re}\left[{#1}\right]}
\newcommand{\diag}{{\rm diag}}
% Derivative
\newcommand{\pdev}[2]{\frac{\partial #1}{\partial #2}}
\newcommand{\dev}[2]{\frac{d\, #1}{d\, #2}}
\newcommand{\del}{\partial}




% List
\newcommand{\blist}[1]{
 \begin{list}{#1}%$\ast\circ\bullet\Right
 \begin{align}
	 arrow
 \end{align}
 $\checkmark\star
  { \setlength{\itemsep}{3pt}
     \setlength{\parsep}{2pt}
     \setlength{\topsep}{3pt}
     \setlength{\partopsep}{0pt}
     \setlength{\leftmargin}{1em}
     \setlength{\labelwidth}{1em}
     \setlength{\labelsep}{0.5em} } }
\newcommand{\elist}{
  \end{list}  }     


\DeclareMathSymbol{\vartheta}{\mathalpha}{letters}{"12}
\DeclareMathSymbol{\theta}{\mathalpha}{letters}{"23}
\DeclareMathSymbol{\phi}{\mathalpha}{letters}{"27}
\DeclareMathSymbol{\varphi}{\mathalpha}{letters}{"1E}

\newcommand{\boxe}[2]
  {
\begin{center}
\noindent\framebox[#2in][c]{\begin{minipage}[c]{\columnwidth}#1\end{minipage}}% 
\end{center}
   }

\newcommand{\boxcolwidth}[1]
  {

   \noindent\fbox{\begin{minipage}[c]{\columnwidth}#1\end{minipage}}  }

\newcommand{\specialcell}[2][c]{%
  \begin{tabular}[#1]{@{}c@{}}#2\end{tabular}}
	
	
\newcommand{\insfigsc}[3]
	{
	\begin{figure}[htbp]
\centering
\includegraphics[width=#3\linewidth]{#1}
\caption{#2}
\zfl{#1}
\end{figure}}

%\newcommand{\insfigscfull}[3]
%	{
%	\begin{figure*}[htbp!]
%\centering
%\includegraphics[width=#3\linewidth]{#1}
%\caption{#2 \zfl{#1}}
%\end{figure*}}


\newcommand{\insfigscfull}[3]
	{
	\begin{figure*}[htbp]
\centering
\includegraphics[width=#3\linewidth]{#1}
\refstepcounter{figure}
\smallskip\noindent\footnotesize  \begin{flushleft} Figure \thefigure: #2\zfl{#1}\end{flushleft}
\end{figure*}}

\newcommand{\bef}
{
\begin{figure}[htbp]
\centering
}

\newcommand{\eef}{\end{figure}}

\newcommand{\subfig}[2]
{
\subfigure[]{\includegraphics[width=#2\linewidth]{#1}\zfl{#1}}
}

%\newcommand{\subfig}[2]
%{
%\subfloat[]{
%\begin{minipage}[c][1\width]{ 0.5\textwidth} 
%\centering	
 %\includegraphics[width=#2\textwidth]{#1} 
%\end{minipage}} 
%\zfl{#1}}


\newcommand{\marfig}[2]
{
\begin{marginfigure}%
\centering
  \includegraphics[width=\linewidth]{#1}
  \caption{#2}
\zfl{#1}
\end{marginfigure}
}

\newcommand{\marfigsc}[3]
{
\begin{marginfigure}%
\centering
  \includegraphics[width=#3\linewidth]{#1}
  \caption{#2}
\zfl{#1}
\end{marginfigure}
}

\newcommand{\beg}{\begingroup
    \fontsize{8pt}{10pt}\selectfont}
\newcommand{\eeg}{\endgroup}
